# Supplementary material for: Minimum Number of k-Cliques in Graphs with Bounded Independence Number
Source: arXiv:1203.4393 ancillary file (2013-04-27)
Supplement: Supplementary file 1 [file Clebsch.pdf]

```

In[1]:= (* binary sequences with even number of 1s *)
v = Select[Tuples[{0, 1}, {5}], EvenQ[Apply[Plus, #]] &]
Out[1]= {{0, 0, 0, 0, 0}, {0, 0, 0, 1, 1}, {0, 0, 1, 0, 1}, {0, 0, 1, 1, 0},
{0, 1, 0, 0, 1}, {0, 1, 0, 1, 0}, {0, 1, 1, 0, 0}, {0, 1, 1, 1, 1},
{1, 0, 0, 0, 1}, {1, 0, 0, 1, 0}, {1, 0, 1, 0, 0}, {1, 0, 1, 1, 1},
{1, 1, 0, 0, 0}, {1, 1, 0, 1, 1}, {1, 1, 1, 0, 1}, {1, 1, 1, 1, 0}}

In[2]:= (* adjacency matrix of Clebsch graph *)
m = Table[
  If[Count[v[[i]] + v[[j]], 1] == 4, 1, 0],
  {i, 16}, {j, 16}]
Out[2]= {{0, 0, 0, 0, 0, 0, 0, 1, 0, 0, 0, 1, 0, 1, 1, 1},
{0, 0, 0, 0, 0, 0, 1, 0, 0, 0, 1, 0, 1, 0, 1, 1},
{0, 0, 0, 0, 0, 1, 0, 0, 0, 1, 0, 0, 1, 1, 0, 1},
{0, 0, 0, 0, 1, 0, 0, 0, 1, 0, 0, 0, 1, 1, 1, 0},
{0, 0, 0, 1, 0, 0, 0, 0, 0, 1, 1, 1, 0, 0, 0, 1},
{0, 0, 1, 0, 0, 0, 0, 0, 1, 0, 1, 1, 0, 0, 1, 0},
{0, 1, 0, 0, 0, 0, 0, 0, 1, 1, 0, 1, 0, 1, 0, 0},
{1, 0, 0, 0, 0, 0, 0, 0, 1, 1, 1, 0, 1, 0, 0, 0},
{0, 0, 0, 1, 0, 1, 1, 1, 0, 0, 0, 0, 0, 0, 0, 1},
{0, 0, 1, 0, 1, 0, 1, 1, 0, 0, 0, 0, 0, 0, 0, 1},
{0, 1, 0, 0, 1, 1, 0, 1, 0, 0, 0, 0, 0, 1, 0, 0},
{1, 0, 0, 0, 1, 1, 1, 0, 0, 0, 0, 0, 1, 0, 0, 0},
{0, 1, 1, 1, 0, 0, 0, 1, 0, 0, 0, 1, 0, 0, 0, 0},
{1, 0, 1, 1, 0, 0, 1, 0, 0, 0, 1, 0, 0, 0, 0, 0},
{1, 1, 0, 1, 0, 1, 0, 0, 0, 1, 0, 0, 0, 0, 0, 0},
{1, 1, 1, 0, 1, 0, 0, 0, 1, 0, 0, 0, 0, 0, 0, 0}}

In[3]:= (* number of k-tuples (v1,...,vk) st v1=1 and they span no edge *)
independent[k_] := independent[k] = Module[{
  p = Tuples[Select[Range[16], m[[1, #]] == 0 &], {k - 1}],
  z = Table[0, {k - 1}, {k - 1}],
  Length[Select[p, (m[[#, #]] == z) &]]
]

In[4]:= independent[6]
Out[4]= 19211

In[5]:= independent[7]
Out[5]= 98491

In[6]:= (* stability for (6,3) and (7,3);
we define p that spans C_5' in the Clebsch graph *)
v[[p = {1, 2, 7, 9, 4, 13}]]
Out[6]= {{0, 0, 0, 0, 0}, {0, 0, 0, 1, 1}, {0, 1, 1, 0, 0},
{1, 0, 0, 0, 1}, {0, 0, 1, 1, 0}, {1, 1, 0, 0, 0}}

In[7]:= (* possible sets Z when we remove z from p except we do not allow z=00000 *)
q = Map[(Complement[p, {#}]) &, {2, 7, 9, 4, 13}]
Out[7]= {{1, 4, 7, 9, 13}, {1, 2, 4, 9, 13}, {1, 2, 4, 7, 13}, {1, 2, 7, 9, 13}, {1, 2, 4, 7, 9}}

In[8]:= (* equivalence s-class *)
equiv[i_Integer, s_List] := Select[Range[16], m[[{i}, s]] == m[[{#}, s]] &]

In[11]:= (* suitable z *)
suitable[i_, j_] := Select[q, (a = m[[equiv[i, #], equiv[j, #]]];
  Max[a] == Min[a]) &];

```

```
In[10]:= (* suitable z with some output information *)
suitablePrint[i_, j_] := (s = Select[q, (a = m[[equiv[i, #], equiv[j, #]]];
    Max[a] == Min[a]) &];
    z = Map[Complement[p, #] &, s];
    Print["x,y: ", v[[i]], " ", v[[j]]];
    Print["List of suitable z: ", Map[v[[#]] &, z]];
    Print["Equivalence classs of x (per each z): ", Map[v[[equiv[i, #]]] &, s]];
    Print["Equivalence classs of y (per each z): ", Map[v[[equiv[j, #]]] &, s]]
)
```

```
In[12]:= (* sample use; this is Row 1 of our table *)
suitablePrint[1, 2]

x,y: {0, 0, 0, 0, 0} {0, 0, 0, 1, 1}

List of suitable z: {{{1, 0, 0, 0, 1}}, {{0, 0, 1, 1, 0}}}

Equivalence classs of x (per each z):
  {{{0, 0, 0, 0, 0}, {0, 1, 0, 1, 0}}, {{0, 0, 0, 0, 0}, {0, 1, 0, 0, 1}}}

Equivalence classs of y (per each z): {{{0, 0, 0, 1, 1}}, {{0, 0, 0, 1, 1}}}
```

```
In[13]:= (* Let us check if z exists for every x,y *)
Table[If[Length[suitable[i, j]] == 0, Print["NO!"]], {i, 16}, {j, i + 1, 16}];
```

```
In[14]:= (* Exact result for (6,3) and (7,3): we compute gradient of X=
{00000, 00011, 00101, 00110} which are vertices labeled 1,2,3,4 wrt m *)
gradient[k_] := gradient[k] = Module[{
    p = Tuples[Range[5, 16], {k - 1}],
    z = Table[0, {k - 1}, {k - 1}],
    Length[Select[p, (m[[#, #]] == z) &]] / 16^(k - 1)
]
```

```
In[15]:= gradient[6]
```

```
Out[15]= 
$$\frac{1437}{65536}$$

```

```
In[16]:= gradient[6] - independent[6] / 16^5
```

```
Out[16]= 
$$\frac{3781}{1048576}$$

```

```
In[17]:= gradient[7]
```

```
Out[17]= 
$$\frac{14503}{2097152}$$

```

```
In[18]:= gradient[7] - independent[6] / 16^6
```

```
Out[18]= 
$$\frac{96813}{16777216}$$

```
